# Supplementary material for: Semantic Segmentation Prior for Diffusion-Based Real-World Super-Resolution
Source: arXiv:2412.02960 source file (2024-12-04)
Supplement: Supplementary file 1 [file X_suppl.tex]

\clearpage
\setcounter{page}{1}
\maketitlesupplementary

In this supplementary file, we provide:
\begin{enumerate}
    \item Detailed information on SegSR, including the training/inference details and setting. 
    \item Architecture details of SegSR. 
    \item Impact of semantic segmentation prior. 
    \item More visual comparison.
    
\end{enumerate}

\section{Detailed Information on SegSR}
\subsection{Training Details on SRDM Branch}
For the SRDM branch, we employ the StableSR~\cite{stablesr} as the baseline, leveraging its pretrained model in conjunction with the Seg Controller within DMB module for joint optimization.
We divide the training process into two progressive stages for Seg Controller that introduce the segmentation prior to SRDM branch. First, to ensure that the segmentation prior can accurately generate corresponding semantic classes and layouts, we train the Seg Controller for stable Seg2Img generation (see Figure~\ref{fig:s2i}), with ControlNet~\cite{controlnet} initialized by cloning the U-Net encoder from the pretrained SD model.
During training, the latent embedding $Z_0$ of the HQ image is obtained by the encoder of pretrained VAE~\cite{sd}. The diffusion process progressively adds noise by following $t$ steps to $Z_0$ to obtain the noisy latent $Z_t$.
Thus, with the noisy segmentation embedding $S_t$, the Seg2Img generator $\epsilon_\theta^1$ predicts the noise $\epsilon$ added to the noisy latent $Z_t$. the training objective $\mathcal{L}_{Seg2Img}$ is formulated as follows:
\begin{equation}
\mathcal{L}_{Seg2Img}=\mathbb{E}_{t,Z_0, S_t,\epsilon\sim\mathcal{N}}\Big[\|\epsilon-\epsilon_\theta^{1}(Z_t,t,S_t))\|_2^2\Big].
\end{equation}

Next, the pretrained Seg Controller is copied to the second stage to incorporate segmentation into the SR process. 
% For the SRDM branch, we employ the StableSR~\cite{stablesr} as the baseline, leveraging its pre-trained model in conjunction with the trained Seg Controller for joint optimization. 
Specifically, similar to the HQ latent $Z_0$, LQ images are processed through the Img Encoder (VAE~\cite{sd}) to derive the LQ latent $Z_{lq}$. This latent $Z_{lq}$ is then fed into the Img Controller (Time-aware Encoder) to obtain the LQ feature condition, which is integrated into the SD for generation guidance via a trainable SFT layer~\cite{sftgan}. 
Therefore, compared to the first stage, the introduction of the additional LQ latent condition $Z_{lq}$ modifies the joint optimization objective of whole network $\epsilon_\theta^{2}$ to $\mathcal{L}_{SR}$:
\begin{equation}
\mathcal{L}_{SR}=\mathbb{E}_{t,Z_0, S_t,Z_{lq},\epsilon\sim\mathcal{N}}\Big[\|\epsilon-\epsilon_\theta^{2}(Z_t,t,S_t,Z_{lq}))\|_2^2\Big].
\end{equation}

% During training, the Seg Controller receives the updated segmentation result $S_t$ from SegDM at $t$ step as input and outputs the Seg feature $C_t$, while the Img Controller (Time-aware Encoder) receives the LQ image latent $Z_{lq}$ to obtain the LQ feature condition, where $S_t$ is detailed in section of Training of SegDM Branch and $Z_{lq}$ is obtained through the Img Encoder (VAE~\cite{sd}) processing LQ image.
% Then,  the Seg feature $C_t$ and LQ feature condition are introduced into the Img Denoiser of SRDM via zero convolution and SFT layers~\cite{sftgan}, respectively. 
% Similar to SD training process, the latent embedding $Z_0$ of the HQ image is obtained by the encoder of pretrained VAE~\cite{sd}, and the diffusion process progressively add noise by following $t$ steps to $Z_0$ to obtain the noisy latent $Z_t$. Thus, the SRDM $\epsilon_\theta$ predict the noise $\epsilon$ added to the noisy latent $Z_t$:
% \begin{equation}
% \mathcal{L}_{SR}=\mathbb{E}_{t,Z_0, S_t,Z_{lq},\epsilon\sim\mathcal{N}}\Big[\|\epsilon-\epsilon_\theta(Z_t,t,S_t,Z_{lq}))\|_2^2\Big].
% \end{equation}

\subsection{Training Details on SegDM Branch}
As predicting semantic segmentation mask from the LQ image is changeling, the training of SegDM goes through two stages. In the first stage, we train a degradation-aware Segformer, consisting of a backbone and a segmentation head, expected to predict coarse segmentation masks on LQ images that approximate the ground-truth masks from HQ images.
In the second stage, inspired by DDPS~\cite{ddps}, we train a discrete diffusion model to capture the distribution of semantic segmentation prior. During training, the ground truth mask is encoded into representation $S_0$ by a Seg Encoder, i.e, a simple resize codec, and then progressively added noise by following $t$ diffusion steps to $S_0$ to obtain the noisy representation $S_t$. Seg Denoiser iteratively denoises $S_t$ to $S_{t-1}$, conditioned on the the backbone features $F_{lq}$ from the first stage. This process can refine the coarse prediction results generated by Segformer. Finally, the logit output can be reconstructed by the Seg Decoder, which performs the reverse operation of the Seg Encoder. Both stages are optimized using the cross-entropy function to compute loss between logit output and ground truth mask, and the training objective of SegDM is formulated as follows:
\begin{equation}
\mathcal{L}_{SegDM}=-\log p_\theta\left(S_0\mid S_t,F_{lq}\right).
\label{eqa:segdm}
\end{equation}

\begin{figure}[!t]
    \centering
    \includegraphics[width=\linewidth]{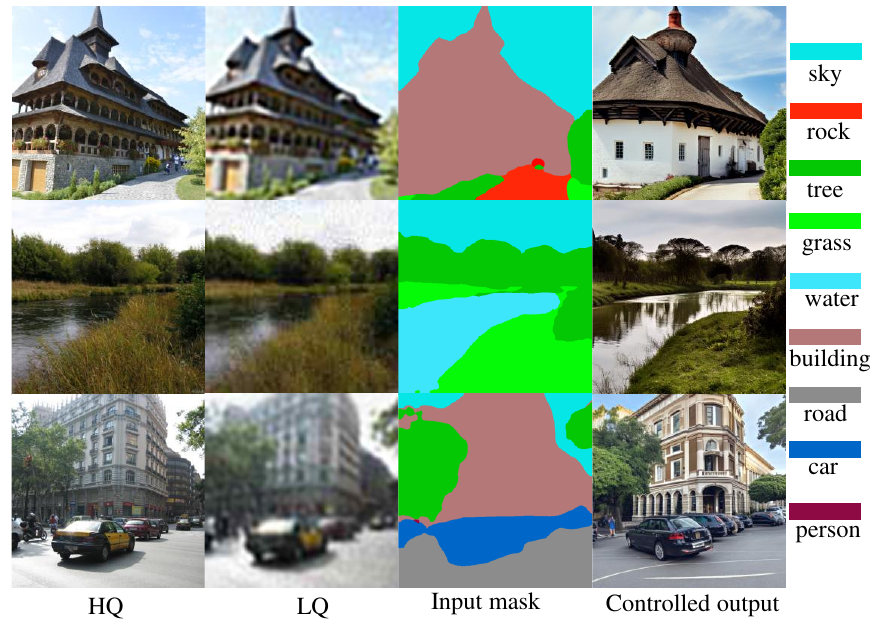}
    \caption{Controlling Stable Diffusion~\cite{sd} with segmentation embedding from SegDM. The third column is the segmentation predictions of SegDM on the LQ images. The last column shows images generated under the guidance of semantic segmentation.}
    \label{fig:s2i}
\end{figure}
\subsection{Joint Training of SegSR Model}
SegSR aims to facilitate mutual refinement between SRDM and SegDM at each diffusion step. Thus, as a bridge connecting the two branches, the DMB needs to be trained jointly with both branches.
For ImgAided Component, we pass the image latent $Z_t$ at $t$ step through it to obtain the restored image information $T_t$, which is then added to the input of Seg Denoiser within SegDM through zero convolution to enhance segmentation prediction. 
Thus, similar to the optimization objective of SegDM at Eq.~\ref{eqa:segdm}, the ImgAided Component is trained using additional updated image latent $Z_t$:
\begin{equation}
\mathcal{L}_{IAC}=-\log p_\theta\left(S_0\mid S_t,F_{lq},Z_t \right).
% \label{eqa:iac}
\end{equation}

For the Seg Controller, we directly copy the pretrained weights of the Seg Controller from the SRDM training stage. Thus, the joint loss function of the whole SegSR framework defined as follows:
\begin{equation}
\mathcal{L}_{SegSR}=\mathcal{L}_{SR}+\lambda\mathcal{L}_{IAC}.
% \label{eqa:iam}
\end{equation}
where $\lambda$ is a balance parameter. The SRDM and SegDM are initialized with the pretrained weights from their respective independent training stages. To save the training cost, the trainable modules include DMB, Time-aware Encoder, and SFT layer within SRDM.

\subsection{Inference Details of SegSR Model}
After introducing SRDM, SegDM, and DMB, the sampling process of SegSR is summarized as follows. Initially, features $Z_{lq}$ and $F_{lq}$ are extracted from the LQ image using the VAE encoder and the backbone of Segformer. The inference process follows a denoising trajectory that begins with the pure noisy latent representation $Z_T$ and mask $S_T$. In the SRDM branch, the Img Denoiser predicts a less noisy latent $Z_{t-1}$ based on $Z_t$, LQ features $Z_{lq}$, and updated segmentation guided condition $C_t$ from the DMB. Simultaneously, the Seg Denoiser estimates the latent state of the segmentation mask $S_{t-1}$, using $S_t$ from the previous step and updated image-guided condition $I_t$ from the DMB. After $T$ collaborative diffusion steps, the final image can be reconstructed through Img decoder.

% Thanks to the joint optimization strategy facilitated by DMB, the proposed SegSR framework can progressively restore realistic images through SRDM, while simultaneously improving the accuracy of semantic segmentation in SegDM.

\subsection{Implementation Details}

All models are trained on LQ-HQ pairs, where the original LQ size of $128\times128\times3$ is resized to match the HQ size of 
$512\times512\times3$. The training details are as follows: \begin{itemize}

    \item Before training SRDM, we first pretrain the Seg Controller in DMB for stable Seg2Img generation. The Seg Controller is trained for 160K iterations with a batch size of 32. The learning rate is fixed at $1\times10^{-5}$ throughout the training process. Subsequently, the Seg Controller and SRDM are jointly trained for another 160K iterations with a fixed learning rate of $5\times10^{-5}$. 
    
    \item Before training SegDM, we first pretrain the semantic segmentation model (SegFormer). The SegFormer model is trained for 160K iterations with a batch size of 16. The learning rate is initialized to $6\times10^{-5}$ and follows a ``poly" LR schedule with a default power factor of 1.0. After pretraining, the SegFormer model is frozen, and the Seg Denoiser in SegDM is trained for 320K iterations with a batch size of 32. Similar to DDPS~\cite{ddps}, the initial learning rate is set to $1.5\times10^{-4}$ and is halved every 20K iterations until it reaches a minimum value of $1\times10^{-6}$. To incorporate updated image conditions, we freeze SegDM and train only the ImgAided Component with a fixed learning rate of $1\times10^{-5}$ and a batch size of 32 for 160K iterations.
    \item Finally, we freeze SegDM branch, and jointly train SRDM and DMB for 320K iterations with a batch size of 32, with a learning rate of $5\times10^{-5}$.
\end{itemize}

Additionally, we employ the Adam optimizer~\cite{adam}, with hyperparameters set to $\beta_1 = 0.9$, $\beta_2 = 0.999$, and a weight decay of 0.01. All experiments are conducted using 8 NVIDIA 32G-A100 GPUs. During training, the diffusion timestep $T$ is set to 1000, while for inference, we adopt the spaced DDIM sampling~\cite{ddim} with 1.0 seta and 50 timesteps. 
\section{Architecture Details of SegSR}
SegSR mainly consists of three parts: SRDM, SegDM, and DMB. The architectural details can be described as follows. 
\begin{itemize}
    \item For the SRDM branch, we adopt StableSR~\cite{stablesr} as the baseline for Real-ISR tasks. The trainable modules include the Img controller (i.e., Time-aware Encoder) and the SFT layer~\cite{sftgan}. The SFT layer integrates the LQ image's representation embedding from Img controller into Img Denoiser (i.e., denoising UNet in StableDiffusion).
    \item For the SegDM branch, we adopt the structure of DDPS~\cite{ddps} for segmentation prior modeling. It consists of three components: a Seg Backbone, a Seg Denoiser, and a mask representation codec. The Seg Backbone, based on Segformer, provides image representations for the initial segmentation predictions. The Seg Denoiser, a variant of U-Net~\cite{unet}, removes noise during the diffusion process. The mask representation codec transforms the segmentation mask into a form that is suitable for generative network processing. In practice, we choose a simple resize codec for its straightforward implementation and computational efficiency.
    \item The DMB module consists of two components: Seg Controller and ImgAided. Specifically, Seg Controller follows the methodology and structure of ControlNet~\cite{controlnet}. It encodes the updated segmentation information from SegDM and injects the encoded information into SRDM via zero convolution. The ImgAided component uses a lightweight U-Net~\cite{sd} to encode the updated image information from SRDM and then adds the encoded information to SegDM.
\end{itemize}
\begin{table}[h!]
\centering
\resizebox{\columnwidth}{!}{%
\begin{tabular}{l|cccc}
\toprule
\multirow{2}{*}{Metrics} & \multicolumn{2}{c}{DIV2K-Val} & \multicolumn{2}{c}{RealSR} \\
\cmidrule(lr){2-3} \cmidrule(lr){4-5}
 & Zero Mask & SegSR & Zero Mask & SegSR \\
\midrule
PSNR $\uparrow$ & 20.26 & 20.42 & 24.55 & 24.61 \\
SSIM $\uparrow$ & 0.4448 & 0.4659 & 0.6774 & 0.6858 \\
LPIPS $\downarrow$ & 0.4026 & 0.3769 & 0.3370 & 0.3434 \\
DISTS $\downarrow$ &0.2407 & 0.2240 & 0.2398 & 0.2349 \\
MUSIQ $\uparrow$ & 69.36 & 72.29 & 64.75 & 67.80 \\
MANIQA $\uparrow$ & 0.4715 & 0.6006 & 0.4387 & 0.5233 \\
CLIPIQA $\uparrow$ & 0.6917 & 0.7723 & 0.6221 & 0.6906 \\
\bottomrule
\end{tabular}}
\caption{Metrics comparison on DIV2K-Val and RealSR datasets.}
\label{tab:zero}
\end{table}

\begin{figure*}[!t]
    \centering
    \includegraphics[width=\linewidth]{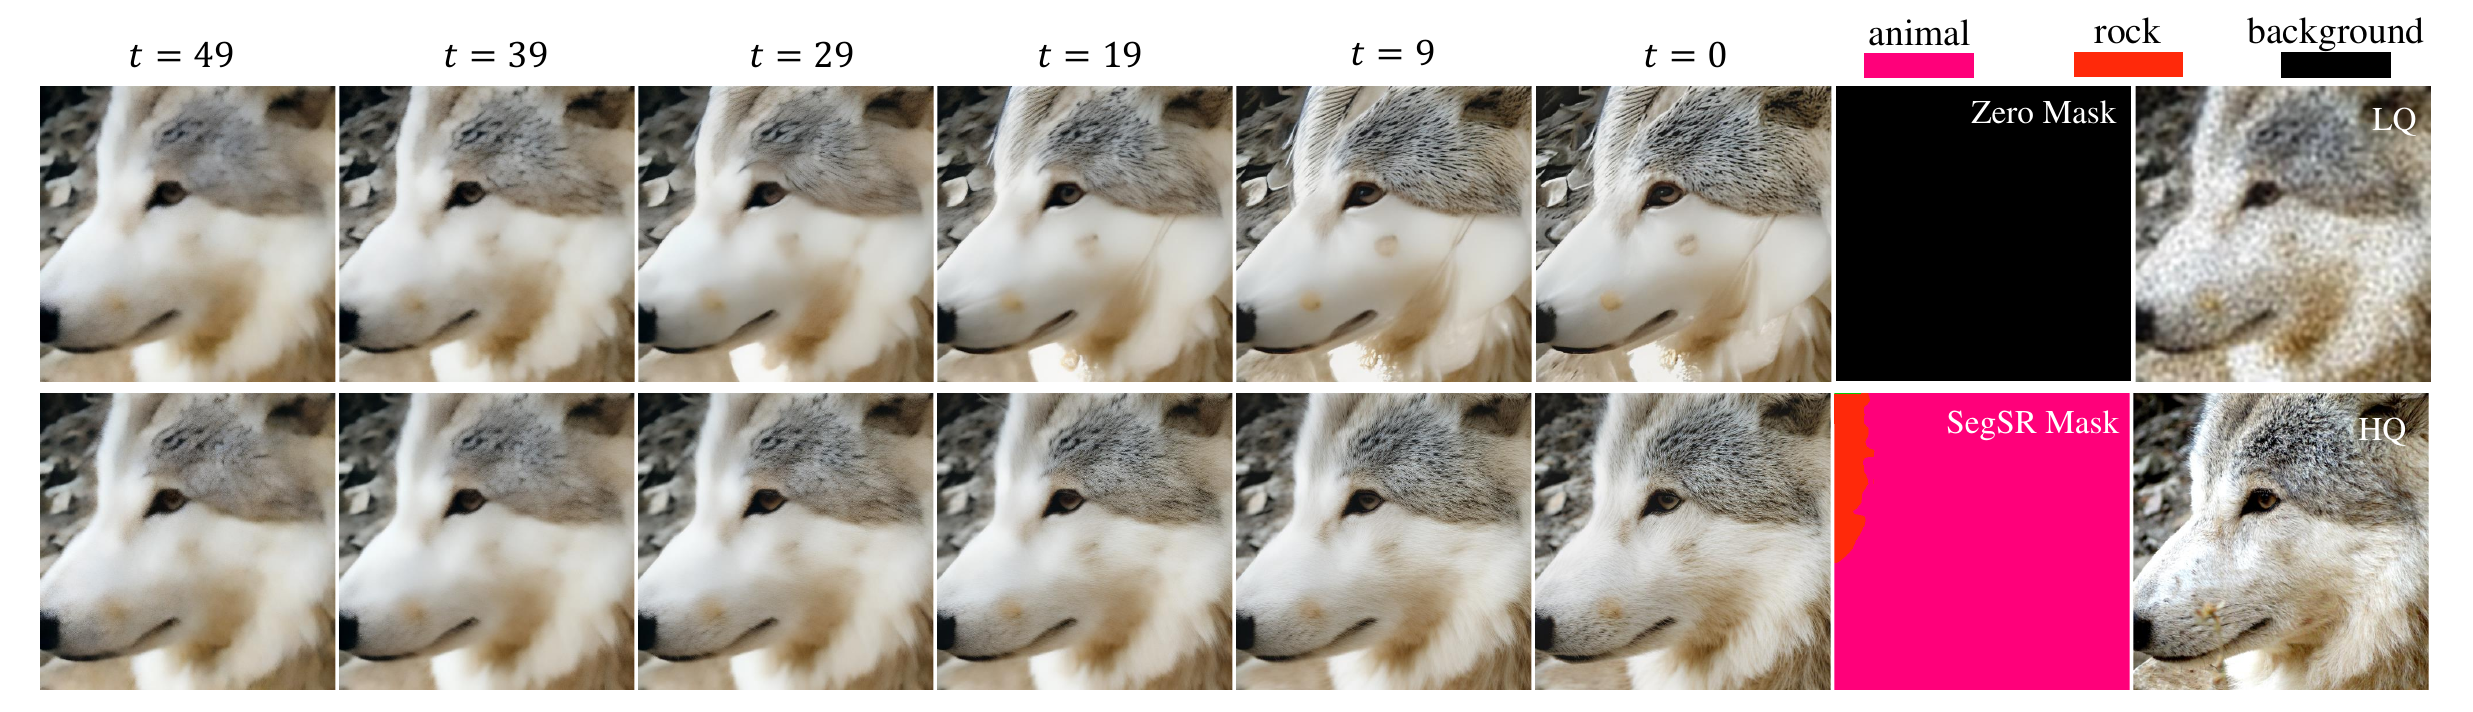}
    \caption{We present the final result predictions at different steps $t$ of the inverse diffusion process, comparing the outcomes using the all-zero mask (top) and our enhanced mask (bottom).}
    \label{fig:zeromap}
\end{figure*}
\def\fwidth{0.16\linewidth}

\begin{figure*}[!ht]
\centering
\begin{tabular}{ccccc}
    % \centering{\rotatebox{90}{  \small{DIV2K-810}}}  \hspace{1pt} &
    % \includegraphics[width=\fwidth]{figs/results/div2k-val/810_color_rect_resize/LQ.png} &  
    % \includegraphics[width=\fwidth]{figs/results/div2k-val/810_color_rect_resize/bsrgan.png} &  
    % \includegraphics[width=\fwidth]{figs/results/div2k-val/810_color_rect_resize/realesrgan.png} &  
    % % \includegraphics[width=\fwidth]{figs/results/div2k-val/810_color_rect_resize/dasr.png} & 
    % \includegraphics[width=\fwidth]{figs/results/div2k-val/810_color_rect_resize/stablesr.png} &  
    % \includegraphics[width=\fwidth]{figs/results/div2k-val/810_color_rect_resize/resshift.png} &  
    % % \includegraphics[width=\fwidth]{figs/results/div2k-val/810_color_rect_resize/pasd.png} & 
    % \includegraphics[width=\fwidth]{figs/results/div2k-val/810_color_rect_resize/diffbir.png} & 
    % \includegraphics[width=\fwidth]{figs/results/div2k-val/810_color_rect_resize/seesr.png} &  
    % \includegraphics[width=\fwidth]{figs/results/div2k-val/810_color_rect_resize/SegSR.png} &
    % \includegraphics[width=\fwidth]{figs/results/div2k-val/810_color_rect_resize/HQ.png} 
    % \\ 
     % \centering{\rotatebox{90}{  \small{DIV2K-844}}}  \hspace{1pt} &
    \includegraphics[width=\fwidth]{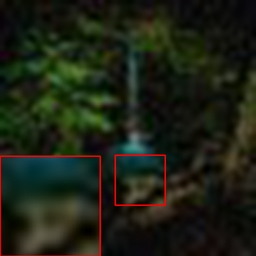} &  
    \includegraphics[width=\fwidth]{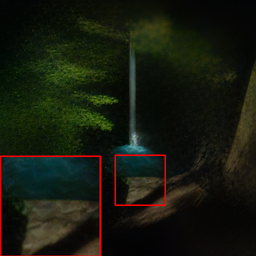} &  
    \includegraphics[width=\fwidth]{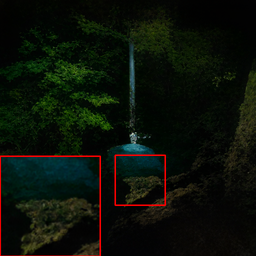} &  
    \includegraphics[width=\fwidth]{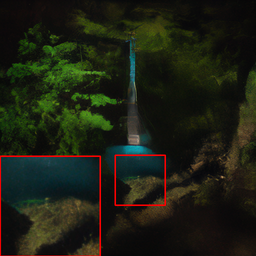} &
     \includegraphics[width=\fwidth]{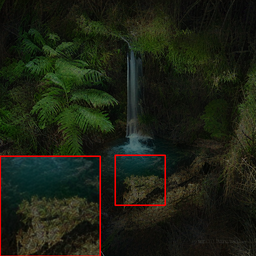} 
    \\ 
       \small{LQ}
    &   \small{BSRGAN}
    &   \small{Real-ESRGAN}
    % &   \small{DASR}
    &   \small{ResShift}
    &   \small{StableSR}
    \\

    \includegraphics[width=\fwidth]{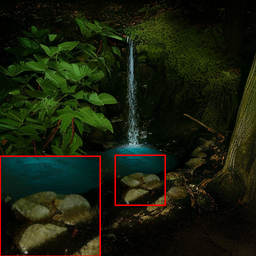} & 
    \includegraphics[width=\fwidth]{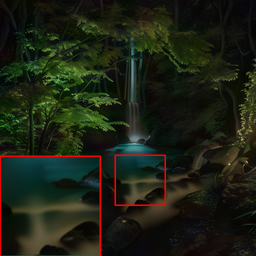} & 
    \includegraphics[width=\fwidth]{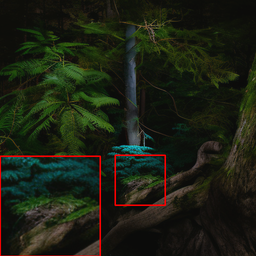} &  
    \includegraphics[width=\fwidth]{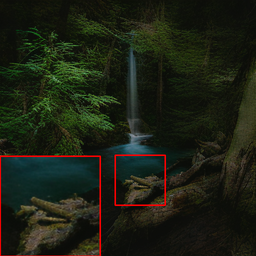} &
    \includegraphics[width=\fwidth]{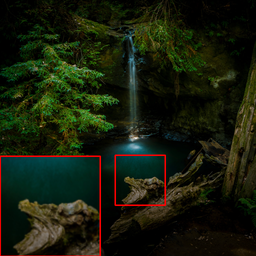} 
    \\
    % &   \small{StableSR}
     \small{DiffBIR}
    &   \small{PASD}
    &   \small{SeeSR}
    &   \small{\textbf{SegSR}}
    &   \small{HQ}
\end{tabular}
\caption{Qualitative comparisons on synthetic benchmark DIV2K-Val~\cite{div2k}. Please zoom in for details.}
\label{fig:qualitative_supp_div2k}
\end{figure*}

\section{Impact of Semantic Segmentation Prior}
    In this work, we define 34 indoor and outdoor categories, including  `sky', `water', `mountain', `building', `sculpture', `road", `grass", `plant', `rock', `vehicle', `animal', `person', `food', `insect', `bird", `boat', `car', `flower', `tree", `book', `bridge', `wall', `fence', `window', `flag', `sand', `furniture', `chair', `table', `dish', `vegetable', `fruit', and `aquatic'. Additionally, a `background' category is introduced to cover regions outside these defined categories.
    
    To evaluate the impact of accurate semantic segmentation guidance, we design experiments comparing the use of our SegSR's segmentation mask versus an all-zero mask, where the all-zero mask represents the "background" category for all pixels. This setup allows us to assess the benefits of detailed semantic information. With the SegSR's mask, the model can leverage accurate semantic labels to better understand object boundaries and spatial structures. In contrast, the all-zero mask eliminates explicit semantic differentiation, treating the entire image as background. The comparison demonstrates how semantic conditioning improves restoration quality and preserves semantic accuracy, as evidenced by superior performance in both quantitative metrics (see Table~\ref{tab:zero}) and visual fidelity (see Figure~\ref{fig:zeromap}).

\def\fwidth{0.16\linewidth}

\begin{figure*}[!ht]
\centering
\begin{tabular}{ccccc}
  
    \includegraphics[width=\fwidth]{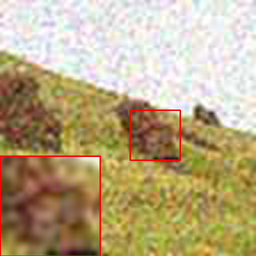} &  
    \includegraphics[width=\fwidth]{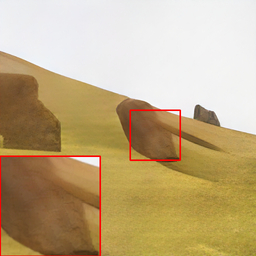} &  
    \includegraphics[width=\fwidth]{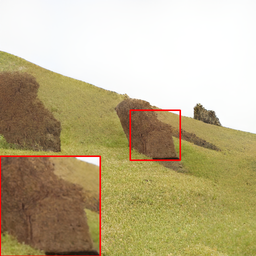} &  
    \includegraphics[width=\fwidth]{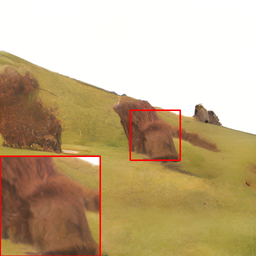}  & 
    \includegraphics[width=\fwidth]{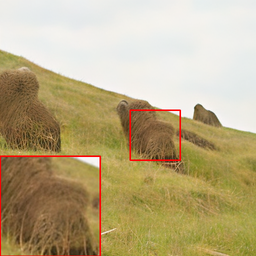} 
        \\ 
       \small{LQ}
    &   \small{BSRGAN}
    &   \small{Real-ESRGAN}
    % &   \small{DASR}
    &   \small{ResShift}
    &   \small{StableSR}
    \\

    \includegraphics[width=\fwidth]{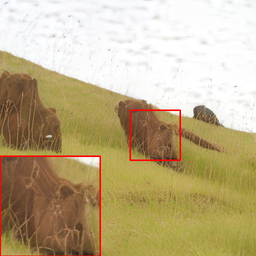} & 
    \includegraphics[width=\fwidth]{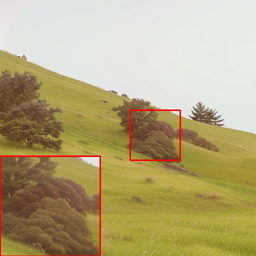} & 
    \includegraphics[width=\fwidth]{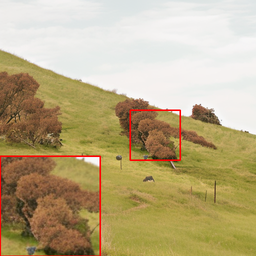} &  
    \includegraphics[width=\fwidth]{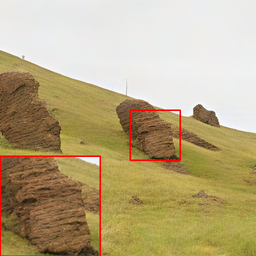} &
    \includegraphics[width=\fwidth]{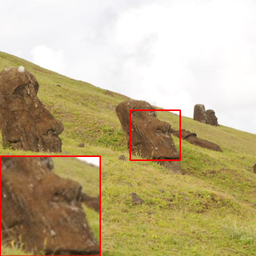} 
     \\ 
     \small{DiffBIR}
    &   \small{PASD}
    &   \small{SeeSR}
    &   \small{\textbf{SegSR}}
    &   \small{HQ}
\end{tabular}
\caption{Qualitative comparisons on synthetic benchmark OST-Val~\cite{sftgan}. Please zoom in for details.}
\label{fig:qualitative_supp_ost}
\end{figure*}

\def\fwidth{0.16\linewidth}

\begin{figure*}[!ht]
\centering
\begin{tabular}{ccccc}

    \includegraphics[width=\fwidth]{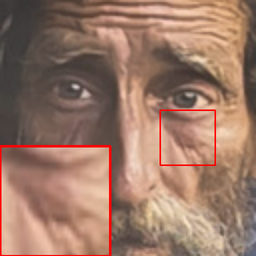} &  
    \includegraphics[width=\fwidth]{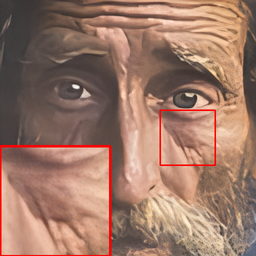} &  
    \includegraphics[width=\fwidth]{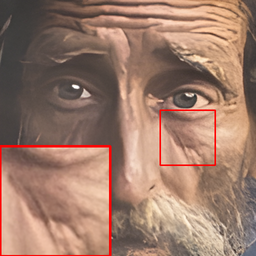} &  
    \includegraphics[width=\fwidth]{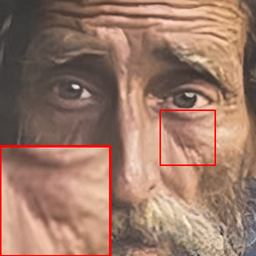} & 
    \includegraphics[width=\fwidth]{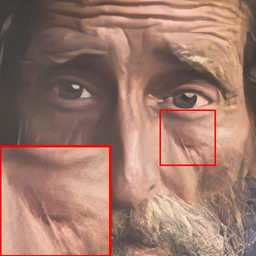} 
        \\ 
       \small{LQ}
     & \small{BSRGAN}
    &   \small{Real-ESRGAN}
    &   \small{DASR}
    &   \small{ResShift}
    \\
     \includegraphics[width=\fwidth]{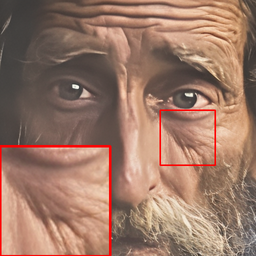} & 
    \includegraphics[width=\fwidth]{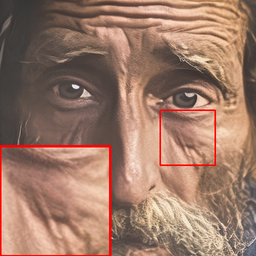} & 
    \includegraphics[width=\fwidth]{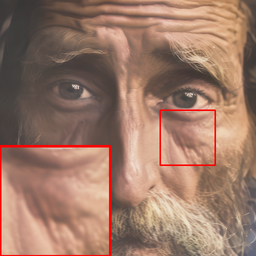} & 
    \includegraphics[width=\fwidth]{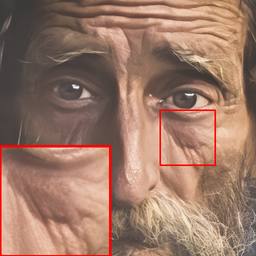} &  
    \includegraphics[width=\fwidth]{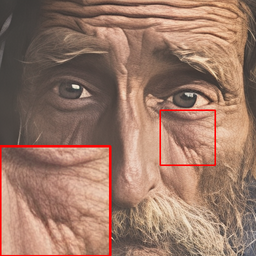} \\

       \small{StableSR}
    &  \small{DiffBIR}
    &   \small{PASD}
    &   \small{SeeSR}
    &   \small{\textbf{SegSR}}
    % &   \small{HQ}
\end{tabular}
\caption{Qualitative comparisons on real-world benchmark RealSR~\cite{realsr}. Please zoom in for details.}
\label{fig:qualitative_supp_realsr}
\end{figure*}

\def\fwidth{0.16\linewidth}

\begin{figure*}[!ht]
\centering
\begin{tabular}{ccccc}

       \includegraphics[width=\fwidth]{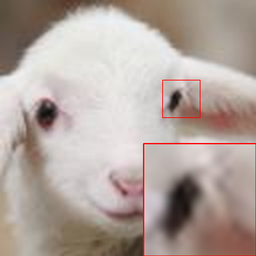} &  
    \includegraphics[width=\fwidth]{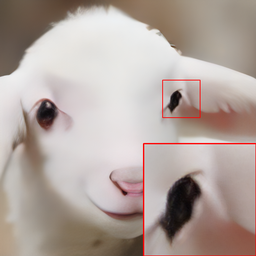} &  
    \includegraphics[width=\fwidth]{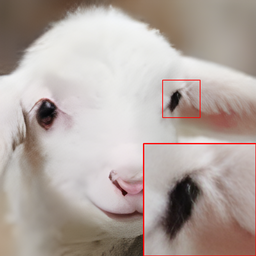} &  
    \includegraphics[width=\fwidth]{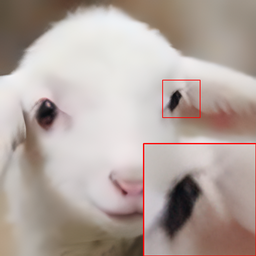} & 
    \includegraphics[width=\fwidth]{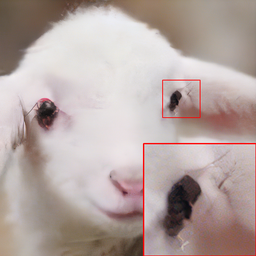} 
        \\ 
       \small{LQ}
     & \small{BSRGAN}
    &   \small{Real-ESRGAN}
    &   \small{DASR}
    &   \small{ResShift}
    \\
     \includegraphics[width=\fwidth]{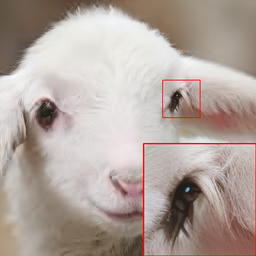} & 
    \includegraphics[width=\fwidth]{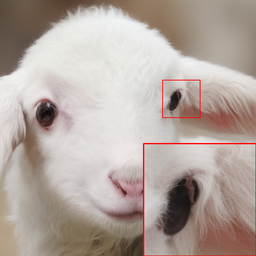} & 
    \includegraphics[width=\fwidth]{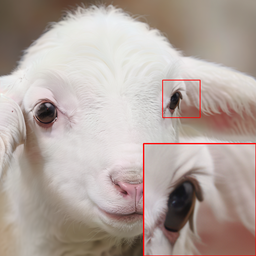} & 
    \includegraphics[width=\fwidth]{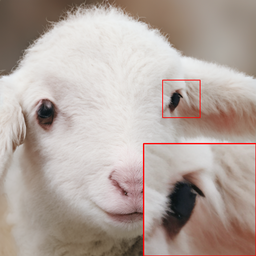} &  
    \includegraphics[width=\fwidth]{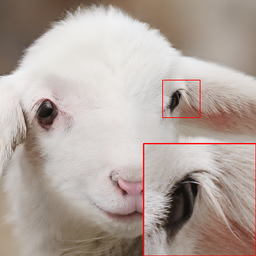} \\

       \small{StableSR}
    &  \small{DiffBIR}
    &   \small{PASD}
    &   \small{SeeSR}
    &   \small{\textbf{SegSR}}
    % &   \small{HQ}
\end{tabular}
\caption{Qualitative comparisons on real-world benchmark RealLQ250~\cite{dreamclear}. Please zoom in for details.}
\label{fig:qualitative_supp_reallq}
\end{figure*}

\section{More visual comparison}
This section presents additional visual results on both synthetic datasets (DIV2K-Val~\cite{div2k} and OST-Val~\cite{sftgan}) and real-world datasets (RealSR~\cite{realsr} and RealLQ250~\cite{drealsr}). SegSR can generate semantically faithful details (the tree and water in Figure~\ref{fig:qualitative_supp_div2k} and the rock in Figure~\ref{fig:qualitative_supp_ost}) and realistic texture (the wrinkle in Figure~\ref{fig:qualitative_supp_realsr} and the wool in Figure~\ref{fig:qualitative_supp_reallq}).
