# Supplementary material for: Semantic Segmentation Prior for Diffusion-Based Real-World Super-Resolution
Source: arXiv:2412.02960 source file (2024-12-04)
Supplement: Supplementary file 2 [file supp_more_fig.tex]

\def\fwidth{0.16\linewidth}

\begin{figure*}[!ht]
\centering
\begin{tabular}{ccccc}
    % \centering{\rotatebox{90}{  \small{DIV2K-810}}}  \hspace{1pt} &
    % \includegraphics[width=\fwidth]{figs/results/div2k-val/810_color_rect_resize/LQ.png} &  
    % \includegraphics[width=\fwidth]{figs/results/div2k-val/810_color_rect_resize/bsrgan.png} &  
    % \includegraphics[width=\fwidth]{figs/results/div2k-val/810_color_rect_resize/realesrgan.png} &  
    % % \includegraphics[width=\fwidth]{figs/results/div2k-val/810_color_rect_resize/dasr.png} & 
    % \includegraphics[width=\fwidth]{figs/results/div2k-val/810_color_rect_resize/stablesr.png} &  
    % \includegraphics[width=\fwidth]{figs/results/div2k-val/810_color_rect_resize/resshift.png} &  
    % % \includegraphics[width=\fwidth]{figs/results/div2k-val/810_color_rect_resize/pasd.png} & 
    % \includegraphics[width=\fwidth]{figs/results/div2k-val/810_color_rect_resize/diffbir.png} & 
    % \includegraphics[width=\fwidth]{figs/results/div2k-val/810_color_rect_resize/seesr.png} &  
    % \includegraphics[width=\fwidth]{figs/results/div2k-val/810_color_rect_resize/SegSR.png} &
    % \includegraphics[width=\fwidth]{figs/results/div2k-val/810_color_rect_resize/HQ.png} 
    % \\ 
     % \centering{\rotatebox{90}{  \small{DIV2K-844}}}  \hspace{1pt} &
    \includegraphics[width=\fwidth]{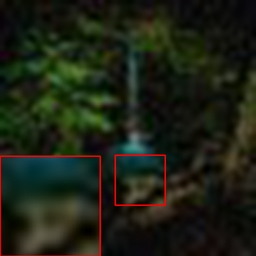} &  
    \includegraphics[width=\fwidth]{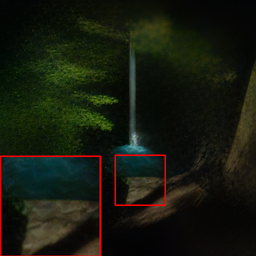} &  
    \includegraphics[width=\fwidth]{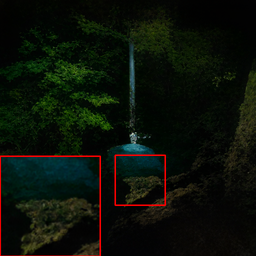} &  
    \includegraphics[width=\fwidth]{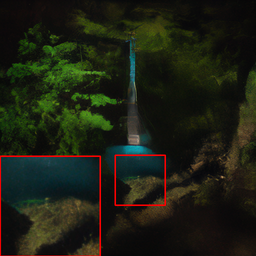} &
     \includegraphics[width=\fwidth]{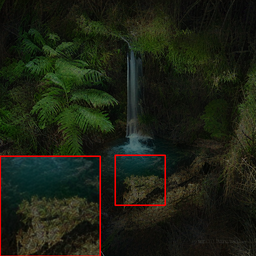} 
    \\ 
       \small{LQ}
    &   \small{BSRGAN}
    &   \small{Real-ESRGAN}
    % &   \small{DASR}
    &   \small{ResShift}
    &   \small{StableSR}
    \\

    \includegraphics[width=\fwidth]{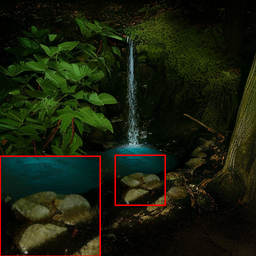} & 
    \includegraphics[width=\fwidth]{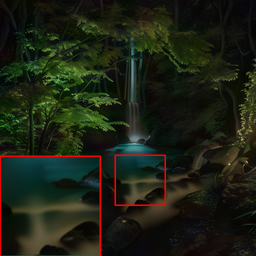} & 
    \includegraphics[width=\fwidth]{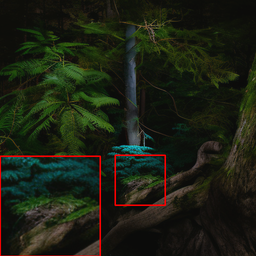} &  
    \includegraphics[width=\fwidth]{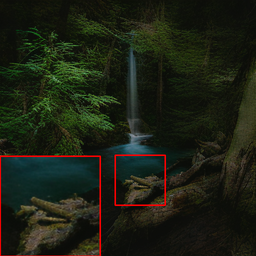} &
    \includegraphics[width=\fwidth]{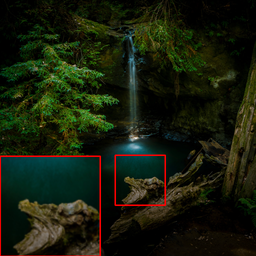} 
    \\
    % &   \small{StableSR}
     \small{DiffBIR}
    &   \small{PASD}
    &   \small{SeeSR}
    &   \small{\textbf{SegSR}}
    &   \small{HQ}
\end{tabular}
\caption{Qualitative comparisons on synthetic benchmark DIV2K-Val~\cite{div2k}. Please zoom in for details.}
\label{fig:qualitative_supp_div2k}
\end{figure*}
