# Supplementary material for: Semantic Segmentation Prior for Diffusion-Based Real-World Super-Resolution
Source: arXiv:2412.02960 source file (2024-12-04)
Supplement: Supplementary file 3 [file supp_more_fig_real.tex]

\def\fwidth{0.16\linewidth}

\begin{figure*}[!ht]
\centering
\begin{tabular}{ccccc}
  
    \includegraphics[width=\fwidth]{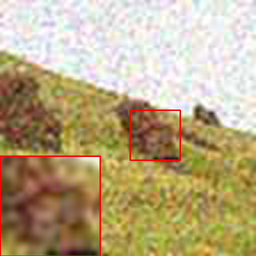} &  
    \includegraphics[width=\fwidth]{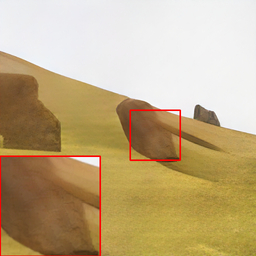} &  
    \includegraphics[width=\fwidth]{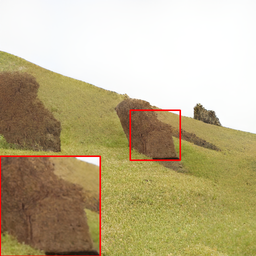} &  
    \includegraphics[width=\fwidth]{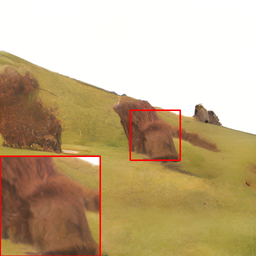}  & 
    \includegraphics[width=\fwidth]{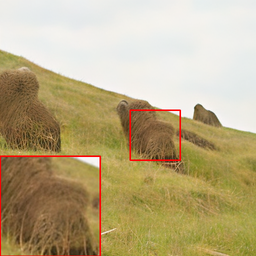} 
        \\ 
       \small{LQ}
    &   \small{BSRGAN}
    &   \small{Real-ESRGAN}
    % &   \small{DASR}
    &   \small{ResShift}
    &   \small{StableSR}
    \\

    \includegraphics[width=\fwidth]{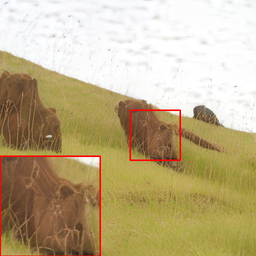} & 
    \includegraphics[width=\fwidth]{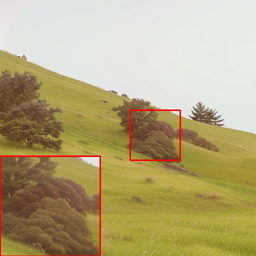} & 
    \includegraphics[width=\fwidth]{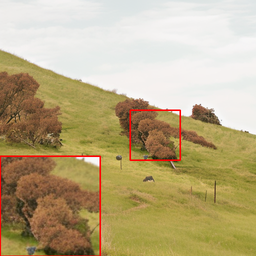} &  
    \includegraphics[width=\fwidth]{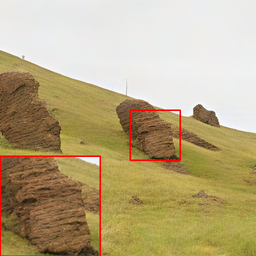} &
    \includegraphics[width=\fwidth]{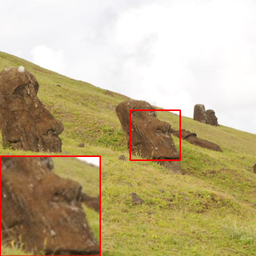} 
     \\ 
     \small{DiffBIR}
    &   \small{PASD}
    &   \small{SeeSR}
    &   \small{\textbf{SegSR}}
    &   \small{HQ}
\end{tabular}
\caption{Qualitative comparisons on synthetic benchmark OST-Val~\cite{sftgan}. Please zoom in for details.}
\label{fig:qualitative_supp_ost}
\end{figure*}

\def\fwidth{0.16\linewidth}

\begin{figure*}[!ht]
\centering
\begin{tabular}{ccccc}

    \includegraphics[width=\fwidth]{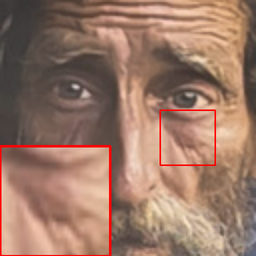} &  
    \includegraphics[width=\fwidth]{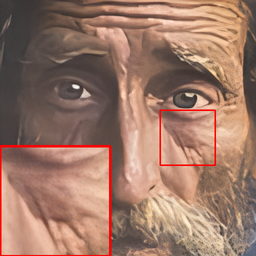} &  
    \includegraphics[width=\fwidth]{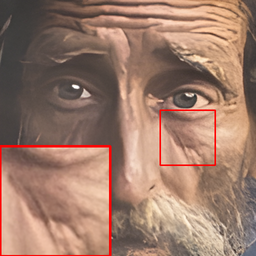} &  
    \includegraphics[width=\fwidth]{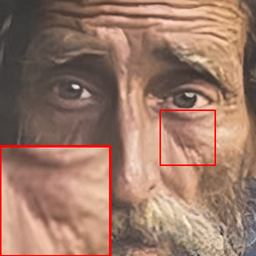} & 
    \includegraphics[width=\fwidth]{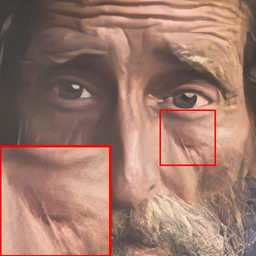} 
        \\ 
       \small{LQ}
     & \small{BSRGAN}
    &   \small{Real-ESRGAN}
    &   \small{DASR}
    &   \small{ResShift}
    \\
     \includegraphics[width=\fwidth]{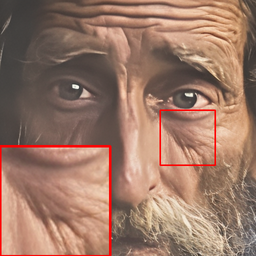} & 
    \includegraphics[width=\fwidth]{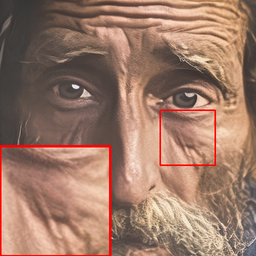} & 
    \includegraphics[width=\fwidth]{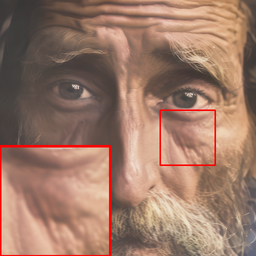} & 
    \includegraphics[width=\fwidth]{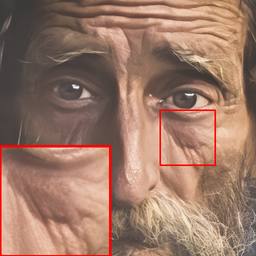} &  
    \includegraphics[width=\fwidth]{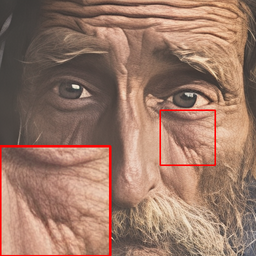} \\

       \small{StableSR}
    &  \small{DiffBIR}
    &   \small{PASD}
    &   \small{SeeSR}
    &   \small{\textbf{SegSR}}
    % &   \small{HQ}
\end{tabular}
\caption{Qualitative comparisons on real-world benchmark RealSR~\cite{realsr}. Please zoom in for details.}
\label{fig:qualitative_supp_realsr}
\end{figure*}

\def\fwidth{0.16\linewidth}

\begin{figure*}[!ht]
\centering
\begin{tabular}{ccccc}

       \includegraphics[width=\fwidth]{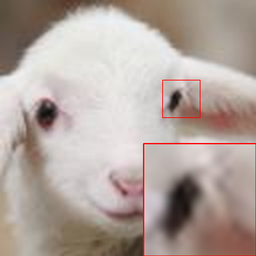} &  
    \includegraphics[width=\fwidth]{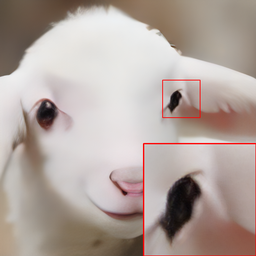} &  
    \includegraphics[width=\fwidth]{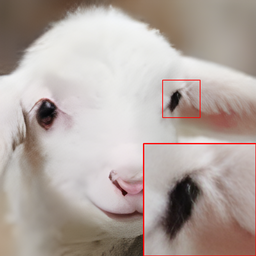} &  
    \includegraphics[width=\fwidth]{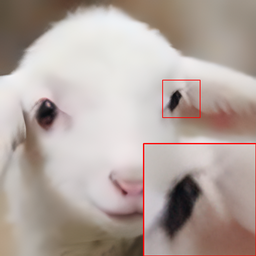} & 
    \includegraphics[width=\fwidth]{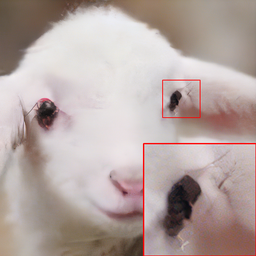} 
        \\ 
       \small{LQ}
     & \small{BSRGAN}
    &   \small{Real-ESRGAN}
    &   \small{DASR}
    &   \small{ResShift}
    \\
     \includegraphics[width=\fwidth]{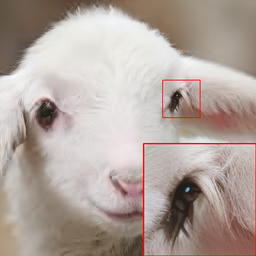} & 
    \includegraphics[width=\fwidth]{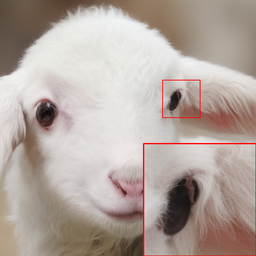} & 
    \includegraphics[width=\fwidth]{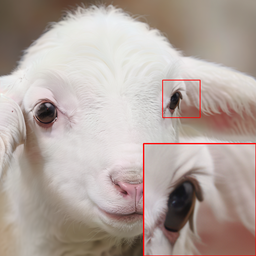} & 
    \includegraphics[width=\fwidth]{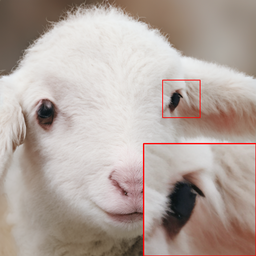} &  
    \includegraphics[width=\fwidth]{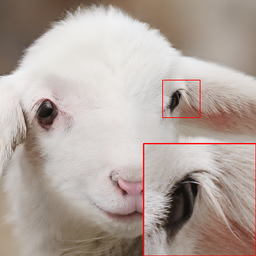} \\

       \small{StableSR}
    &  \small{DiffBIR}
    &   \small{PASD}
    &   \small{SeeSR}
    &   \small{\textbf{SegSR}}
    % &   \small{HQ}
\end{tabular}
\caption{Qualitative comparisons on real-world benchmark RealLQ250~\cite{dreamclear}. Please zoom in for details.}
\label{fig:qualitative_supp_reallq}
\end{figure*}
